# Supplementary material for: DeepCut: Joint Subset Partition and Labeling for Multi Person Pose Estimation
Source: arXiv:1511.06645 source file (2016-04-26)
Supplement: Supplementary file 1 [file figure_qualitative_mpii_supplemental_all.tex]

\begin{figure*}
  \centering
  \begin{tabular}{c c c c c c}

\includegraphics[width=0.16\linewidth]{figures/mpii-supp/imgidx_0013_init_graph.pdf}&
\includegraphics[width=0.16\linewidth]{figures/mpii-supp/imgidx_0013_graph.pdf}&
\includegraphics[width=0.16\linewidth]{figures/mpii-supp/imgidx_0013_sticks.pdf}&

\includegraphics[width=0.16\linewidth]{figures/mpii-supp/imgidx_0231_init_graph.pdf}&
\includegraphics[width=0.16\linewidth]{figures/mpii-supp/imgidx_0231_graph.pdf}&
\includegraphics[width=0.16\linewidth]{figures/mpii-supp/imgidx_0231_sticks.pdf}\\

\includegraphics[width=0.16\linewidth]{figures/mpii-supp/imgidx_0405_init_graph.pdf}&
\includegraphics[width=0.16\linewidth]{figures/mpii-supp/imgidx_0405_graph.pdf}&
\includegraphics[width=0.16\linewidth]{figures/mpii-supp/imgidx_0405_sticks.pdf}&

\includegraphics[width=0.16\linewidth]{figures/mpii-supp/imgidx_0564_init_graph.pdf}&
\includegraphics[width=0.16\linewidth]{figures/mpii-supp/imgidx_0564_graph.pdf}&
\includegraphics[width=0.16\linewidth]{figures/mpii-supp/imgidx_0564_sticks.pdf}\\

\includegraphics[width=0.16\linewidth]{figures/mpii-supp/imgidx_0630_init_graph.pdf}&
\includegraphics[width=0.16\linewidth]{figures/mpii-supp/imgidx_0630_graph.pdf}&
\includegraphics[width=0.16\linewidth]{figures/mpii-supp/imgidx_0630_sticks.pdf}&

\includegraphics[width=0.16\linewidth]{figures/mpii-supp/imgidx_0953_init_graph.pdf}&
\includegraphics[width=0.16\linewidth]{figures/mpii-supp/imgidx_0953_graph.pdf}&
\includegraphics[width=0.16\linewidth]{figures/mpii-supp/imgidx_0953_sticks.pdf}\\

\includegraphics[width=0.16\linewidth]{figures/mpii-supp/imgidx_0960_init_graph.pdf}&
\includegraphics[width=0.16\linewidth]{figures/mpii-supp/imgidx_0960_graph.pdf}&
\includegraphics[width=0.16\linewidth]{figures/mpii-supp/imgidx_0960_sticks.pdf}&

\includegraphics[width=0.16\linewidth]{figures/mpii-supp/imgidx_1025_init_graph.pdf}&
\includegraphics[width=0.16\linewidth]{figures/mpii-supp/imgidx_1025_graph.pdf}&
\includegraphics[width=0.16\linewidth]{figures/mpii-supp/imgidx_1025_sticks.pdf}\\

\includegraphics[width=0.16\linewidth]{figures/mpii-supp/imgidx_1620_init_graph.pdf}&
\includegraphics[width=0.16\linewidth]{figures/mpii-supp/imgidx_1620_graph.pdf}&
\includegraphics[width=0.16\linewidth]{figures/mpii-supp/imgidx_1620_sticks.pdf}&

\includegraphics[width=0.16\linewidth]{figures/mpii-supp/imgidx_1621_init_graph.pdf}&
\includegraphics[width=0.16\linewidth]{figures/mpii-supp/imgidx_1621_graph.pdf}&
\includegraphics[width=0.16\linewidth]{figures/mpii-supp/imgidx_1621_sticks.pdf}\\

\includegraphics[width=0.16\linewidth]{figures/mpii-supp/imgidx_0488_init_graph.pdf}&
\includegraphics[width=0.16\linewidth]{figures/mpii-supp/imgidx_0488_graph.pdf}&
\includegraphics[width=0.16\linewidth]{figures/mpii-supp/imgidx_0488_sticks.pdf}&

\includegraphics[width=0.16\linewidth]{figures/mpii-supp/imgidx_0311_init_graph.pdf}&
\includegraphics[width=0.16\linewidth]{figures/mpii-supp/imgidx_0311_graph.pdf}&
\includegraphics[width=0.16\linewidth]{figures/mpii-supp/imgidx_0311_sticks.pdf}\\

\includegraphics[width=0.16\linewidth]{figures/mpii-supp/imgidx_1680_init_graph.pdf}&
\includegraphics[width=0.16\linewidth]{figures/mpii-supp/imgidx_1680_graph.pdf}&
\includegraphics[width=0.16\linewidth]{figures/mpii-supp/imgidx_1680_sticks.pdf}&

\includegraphics[width=0.16\linewidth]{figures/mpii-supp/imgidx_1692_init_graph.pdf}&
\includegraphics[width=0.16\linewidth]{figures/mpii-supp/imgidx_1692_graph.pdf}&
\includegraphics[width=0.16\linewidth]{figures/mpii-supp/imgidx_1692_sticks.pdf}\\

  \end{tabular}
  \label{fig:qualitative_mpii}
\end{figure*}

\begin{figure*}
  \centering
  \begin{tabular}{c c c c c c}

\includegraphics[width=0.16\linewidth]{figures/mpii-supp/imgidx_0695_init_graph.pdf}&
\includegraphics[width=0.16\linewidth]{figures/mpii-supp/imgidx_0695_graph.pdf}&
\includegraphics[width=0.16\linewidth]{figures/mpii-supp/imgidx_0695_sticks.pdf}&

\includegraphics[width=0.16\linewidth]{figures/mpii-supp/imgidx_1346_init_graph.pdf}&
\includegraphics[width=0.16\linewidth]{figures/mpii-supp/imgidx_1346_graph.pdf}&
\includegraphics[width=0.16\linewidth]{figures/mpii-supp/imgidx_1346_sticks.pdf}\\

\includegraphics[width=0.16\linewidth]{figures/mpii-supp/imgidx_1253_init_graph.pdf}&
\includegraphics[width=0.16\linewidth]{figures/mpii-supp/imgidx_1253_graph.pdf}&
\includegraphics[width=0.16\linewidth]{figures/mpii-supp/imgidx_1253_sticks.pdf}&

\includegraphics[width=0.16\linewidth]{figures/mpii-supp/imgidx_1674_init_graph.pdf}&
\includegraphics[width=0.16\linewidth]{figures/mpii-supp/imgidx_1674_graph.pdf}&
\includegraphics[width=0.16\linewidth]{figures/mpii-supp/imgidx_1674_sticks.pdf}\\

\includegraphics[width=0.16\linewidth]{figures/mpii-supp/imgidx_0908_init_graph.pdf}&
\includegraphics[width=0.16\linewidth]{figures/mpii-supp/imgidx_0908_graph.pdf}&
\includegraphics[width=0.16\linewidth]{figures/mpii-supp/imgidx_0908_sticks.pdf}&

\includegraphics[width=0.16\linewidth]{figures/mpii-supp/imgidx_0104_init_graph.pdf}&
\includegraphics[width=0.16\linewidth]{figures/mpii-supp/imgidx_0104_graph.pdf}&
\includegraphics[width=0.16\linewidth]{figures/mpii-supp/imgidx_0104_sticks.pdf}\\

\includegraphics[width=0.16\linewidth]{figures/mpii-supp/imgidx_0326_init_graph.pdf}&
\includegraphics[width=0.16\linewidth]{figures/mpii-supp/imgidx_0326_graph.pdf}&
\includegraphics[width=0.16\linewidth]{figures/mpii-supp/imgidx_0326_sticks.pdf}&

\includegraphics[width=0.16\linewidth]{figures/mpii-supp/imgidx_0330_init_graph.pdf}&
\includegraphics[width=0.16\linewidth]{figures/mpii-supp/imgidx_0330_graph.pdf}&
\includegraphics[width=0.16\linewidth]{figures/mpii-supp/imgidx_0330_sticks.pdf}\\

\includegraphics[width=0.16\linewidth]{figures/mpii-supp/imgidx_1097_init_graph.pdf}&
\includegraphics[width=0.16\linewidth]{figures/mpii-supp/imgidx_1097_graph.pdf}&
\includegraphics[width=0.16\linewidth]{figures/mpii-supp/imgidx_1097_sticks.pdf}&

\includegraphics[width=0.16\linewidth]{figures/mpii-supp/imgidx_1017_init_graph.pdf}&
\includegraphics[width=0.16\linewidth]{figures/mpii-supp/imgidx_1017_graph.pdf}&
\includegraphics[width=0.16\linewidth]{figures/mpii-supp/imgidx_1017_sticks.pdf}\\

\includegraphics[width=0.16\linewidth]{figures/mpii-supp/imgidx_0950_init_graph.pdf}&
\includegraphics[width=0.16\linewidth]{figures/mpii-supp/imgidx_0950_graph.pdf}&
\includegraphics[width=0.16\linewidth]{figures/mpii-supp/imgidx_0950_sticks.pdf}&

\includegraphics[width=0.16\linewidth]{figures/mpii-supp/imgidx_1652_init_graph.pdf}&
\includegraphics[width=0.16\linewidth]{figures/mpii-supp/imgidx_1652_graph.pdf}&
\includegraphics[width=0.16\linewidth]{figures/mpii-supp/imgidx_1652_sticks.pdf}\\

\includegraphics[width=0.16\linewidth]{figures/mpii-supp/imgidx_0568_init_graph.pdf}&
\includegraphics[width=0.16\linewidth]{figures/mpii-supp/imgidx_0568_graph.pdf}&
\includegraphics[width=0.16\linewidth]{figures/mpii-supp/imgidx_0568_sticks.pdf}&

\includegraphics[width=0.16\linewidth]{figures/mpii-supp/imgidx_0629_init_graph.pdf}&
\includegraphics[width=0.16\linewidth]{figures/mpii-supp/imgidx_0629_graph.pdf}&
\includegraphics[width=0.16\linewidth]{figures/mpii-supp/imgidx_0629_sticks.pdf}\\

\includegraphics[width=0.16\linewidth]{figures/mpii-supp/imgidx_1589_init_graph.pdf}&
\includegraphics[width=0.16\linewidth]{figures/mpii-supp/imgidx_1589_graph.pdf}&
\includegraphics[width=0.16\linewidth]{figures/mpii-supp/imgidx_1589_sticks.pdf}&

\includegraphics[width=0.16\linewidth]{figures/mpii-supp/imgidx_1183_init_graph.pdf}&
\includegraphics[width=0.16\linewidth]{figures/mpii-supp/imgidx_1183_graph.pdf}&
\includegraphics[width=0.16\linewidth]{figures/mpii-supp/imgidx_1183_sticks.pdf}\\

\includegraphics[width=0.16\linewidth]{figures/mpii-supp/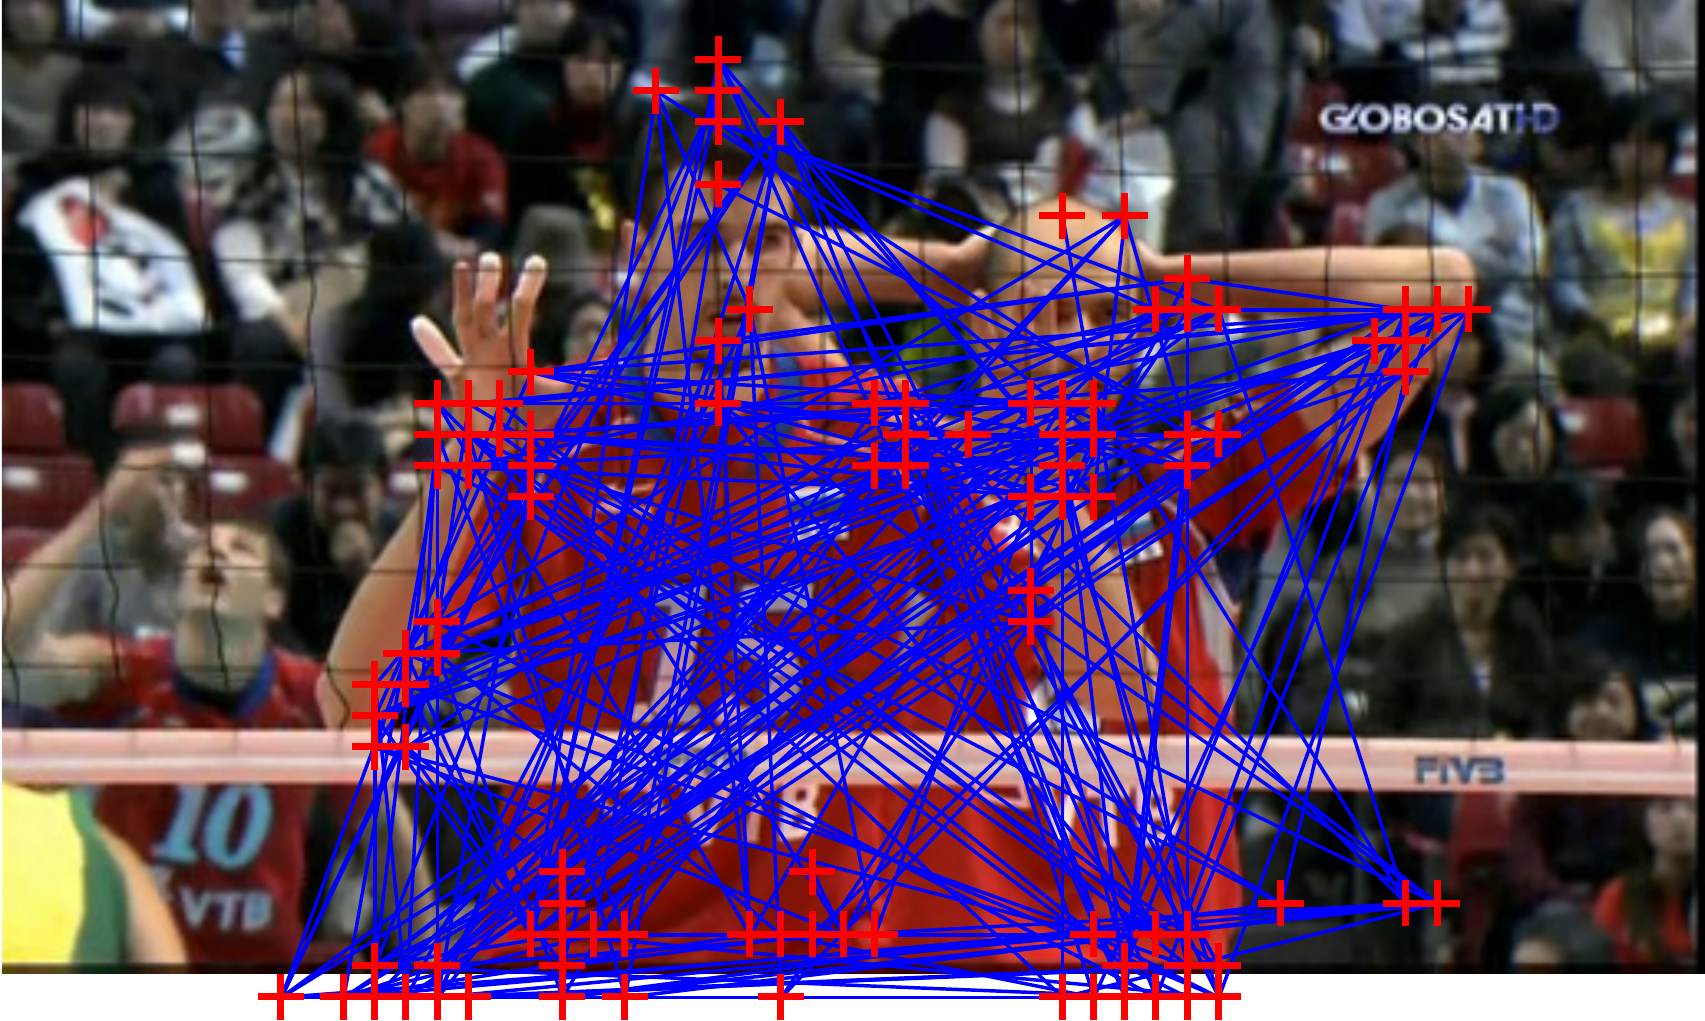}&
\includegraphics[width=0.16\linewidth]{figures/mpii-supp/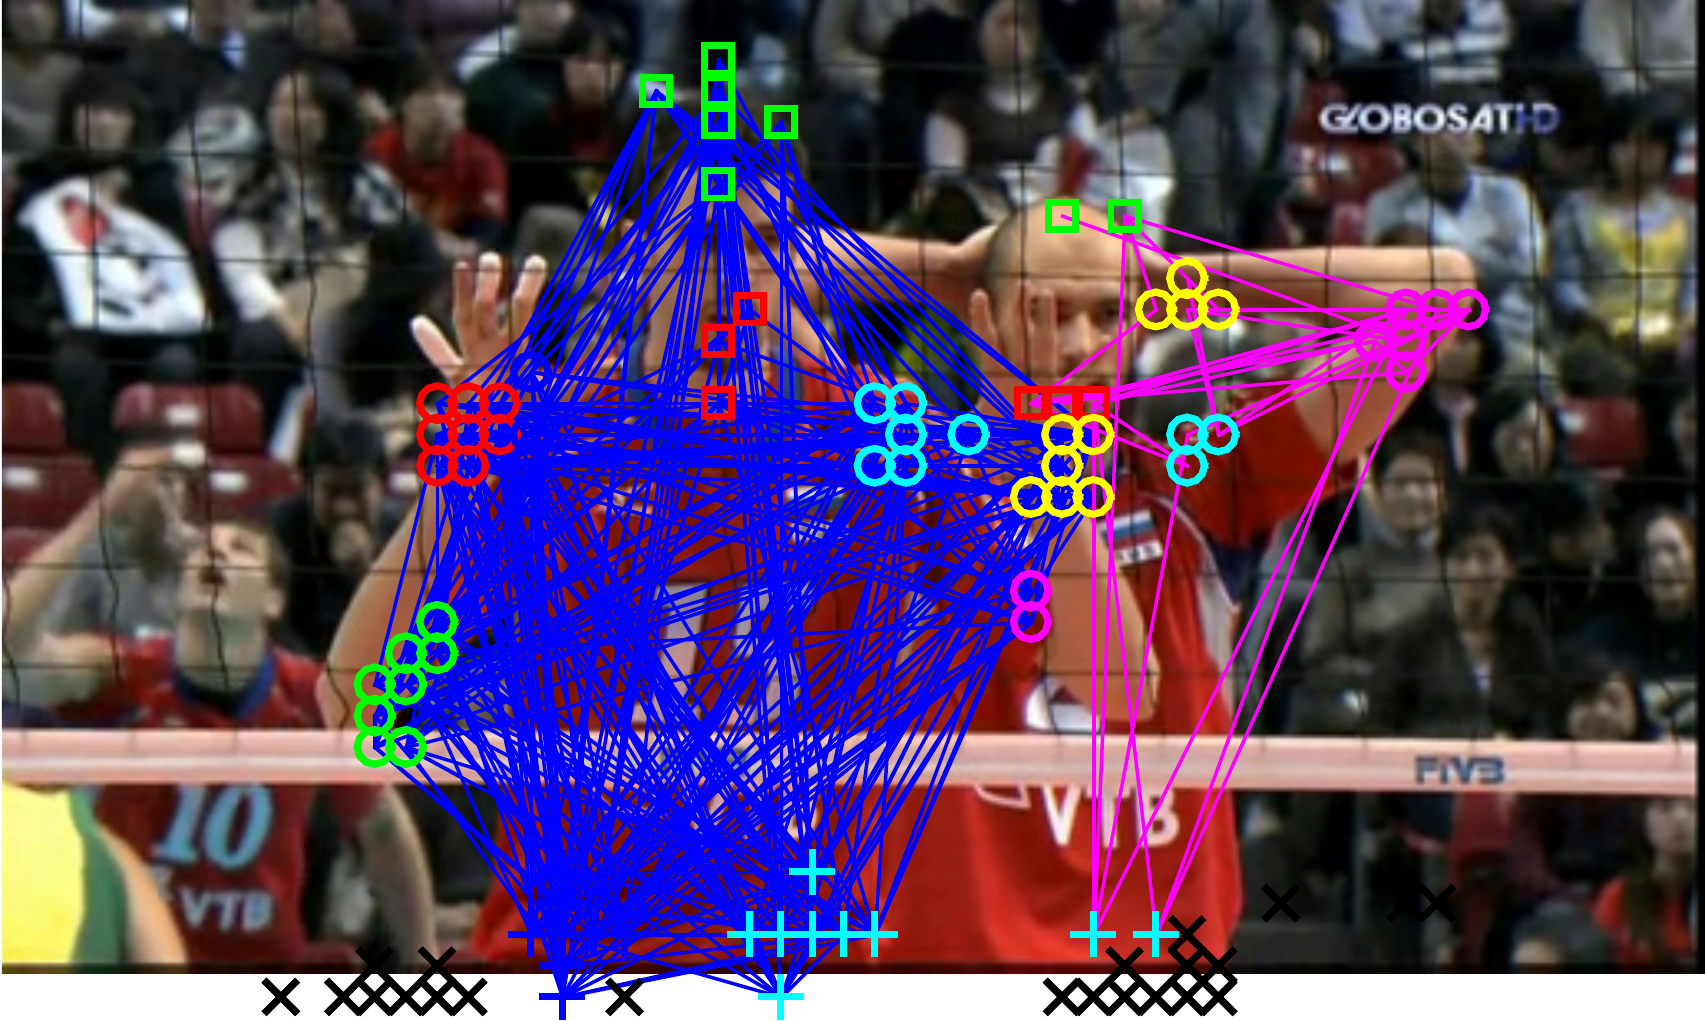}&
\includegraphics[width=0.16\linewidth]{figures/mpii-supp/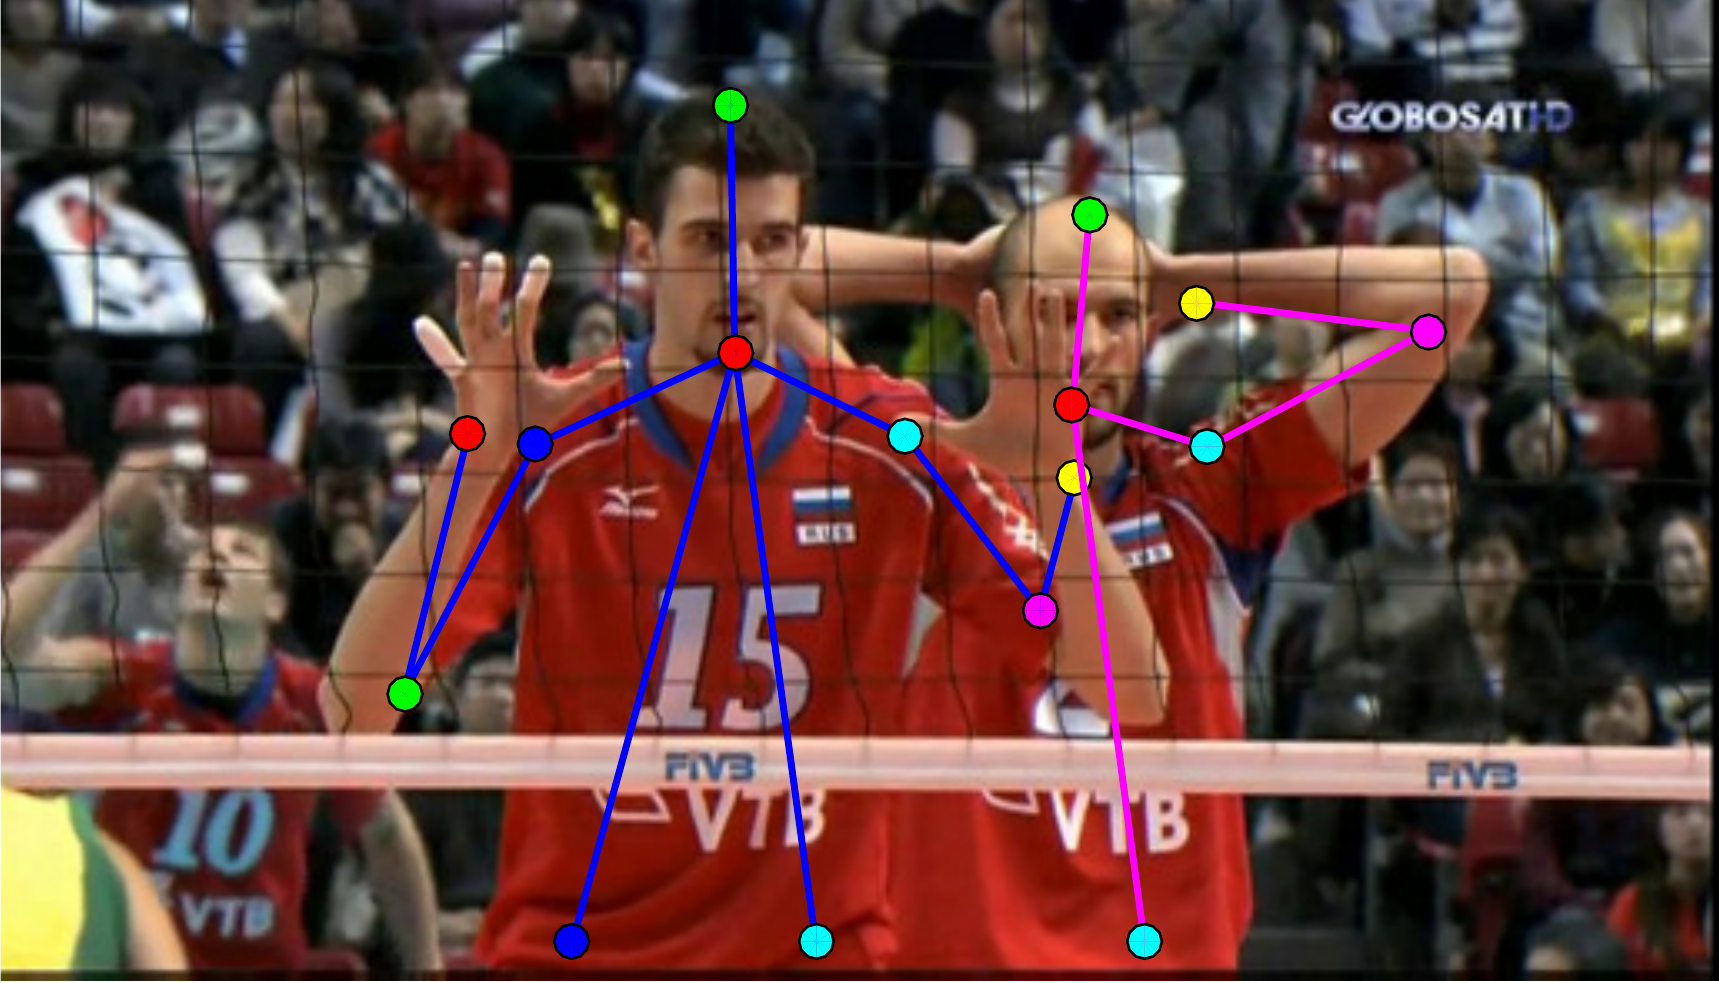}&

\includegraphics[width=0.16\linewidth]{figures/mpii-supp/imgidx_1366_init_graph.pdf}&
\includegraphics[width=0.16\linewidth]{figures/mpii-supp/imgidx_1366_graph.pdf}&
\includegraphics[width=0.16\linewidth]{figures/mpii-supp/imgidx_1366_sticks.pdf}\\

  \end{tabular}
  \label{fig:qualitative_mpii_2}
\end{figure*}

\begin{figure*}
  \centering
  \begin{tabular}{c c c c c c}

\includegraphics[width=0.16\linewidth]{figures/mpii-supp/imgidx_0029_init_graph.pdf}&
\includegraphics[width=0.16\linewidth]{figures/mpii-supp/imgidx_0029_graph.pdf}&
\includegraphics[width=0.16\linewidth]{figures/mpii-supp/imgidx_0029_sticks.pdf}&

\includegraphics[width=0.16\linewidth]{figures/mpii-supp/imgidx_0772_init_graph.pdf}&
\includegraphics[width=0.16\linewidth]{figures/mpii-supp/imgidx_0772_graph.pdf}&
\includegraphics[width=0.16\linewidth]{figures/mpii-supp/imgidx_0772_sticks.pdf}\\

\includegraphics[width=0.16\linewidth]{figures/mpii-supp/imgidx_0832_init_graph.pdf}&
\includegraphics[width=0.16\linewidth]{figures/mpii-supp/imgidx_0832_graph.pdf}&
\includegraphics[width=0.16\linewidth]{figures/mpii-supp/imgidx_0832_sticks.pdf}&

\includegraphics[width=0.16\linewidth]{figures/mpii-supp/imgidx_0635_init_graph.pdf}&
\includegraphics[width=0.16\linewidth]{figures/mpii-supp/imgidx_0635_graph.pdf}&
\includegraphics[width=0.16\linewidth]{figures/mpii-supp/imgidx_0635_sticks.pdf}\\

\includegraphics[width=0.16\linewidth]{figures/mpii-supp/imgidx_0170_init_graph.pdf}&
\includegraphics[width=0.16\linewidth]{figures/mpii-supp/imgidx_0170_graph.pdf}&
\includegraphics[width=0.16\linewidth]{figures/mpii-supp/imgidx_0170_sticks.pdf}&

\includegraphics[width=0.16\linewidth]{figures/mpii-supp/imgidx_0006_init_graph.pdf}&
\includegraphics[width=0.16\linewidth]{figures/mpii-supp/imgidx_0006_graph.pdf}&
\includegraphics[width=0.16\linewidth]{figures/mpii-supp/imgidx_0006_sticks.pdf}\\

\includegraphics[width=0.16\linewidth]{figures/mpii-supp/imgidx_0094_init_graph.pdf}&
\includegraphics[width=0.16\linewidth]{figures/mpii-supp/imgidx_0094_graph.pdf}&
\includegraphics[width=0.16\linewidth]{figures/mpii-supp/imgidx_0094_sticks.pdf}&

\includegraphics[width=0.16\linewidth]{figures/mpii-supp/imgidx_0903_init_graph.pdf}&
\includegraphics[width=0.16\linewidth]{figures/mpii-supp/imgidx_0903_graph.pdf}&
\includegraphics[width=0.16\linewidth]{figures/mpii-supp/imgidx_0903_sticks.pdf}\\

\includegraphics[width=0.16\linewidth]{figures/mpii-supp/imgidx_1116_init_graph.pdf}&
\includegraphics[width=0.16\linewidth]{figures/mpii-supp/imgidx_1116_graph.pdf}&
\includegraphics[width=0.16\linewidth]{figures/mpii-supp/imgidx_1116_sticks.pdf}&

\includegraphics[width=0.16\linewidth]{figures/mpii-supp/imgidx_0697_init_graph.pdf}&
\includegraphics[width=0.16\linewidth]{figures/mpii-supp/imgidx_0697_graph.pdf}&
\includegraphics[width=0.16\linewidth]{figures/mpii-supp/imgidx_0697_sticks.pdf}\\

\includegraphics[width=0.16\linewidth]{figures/mpii-supp/imgidx_0210_init_graph.pdf}&
\includegraphics[width=0.16\linewidth]{figures/mpii-supp/imgidx_0210_graph.pdf}&
\includegraphics[width=0.16\linewidth]{figures/mpii-supp/imgidx_0210_sticks.pdf}&

\includegraphics[width=0.16\linewidth]{figures/mpii-supp/imgidx_1033_init_graph.pdf}&
\includegraphics[width=0.16\linewidth]{figures/mpii-supp/imgidx_1033_graph.pdf}&
\includegraphics[width=0.16\linewidth]{figures/mpii-supp/imgidx_1033_sticks.pdf}\\

\includegraphics[width=0.16\linewidth]{figures/mpii-supp/imgidx_0804_init_graph.pdf}&
\includegraphics[width=0.16\linewidth]{figures/mpii-supp/imgidx_0804_graph.pdf}&
\includegraphics[width=0.16\linewidth]{figures/mpii-supp/imgidx_0804_sticks.pdf}&

\includegraphics[width=0.16\linewidth]{figures/mpii-supp/imgidx_0704_init_graph.pdf}&
\includegraphics[width=0.16\linewidth]{figures/mpii-supp/imgidx_0704_graph.pdf}&
\includegraphics[width=0.16\linewidth]{figures/mpii-supp/imgidx_0704_sticks.pdf}\\

\includegraphics[width=0.16\linewidth]{figures/mpii-supp/imgidx_0075_init_graph.pdf}&
\includegraphics[width=0.16\linewidth]{figures/mpii-supp/imgidx_0075_graph.pdf}&
\includegraphics[width=0.16\linewidth]{figures/mpii-supp/imgidx_0075_sticks.pdf}&

\includegraphics[width=0.16\linewidth]{figures/mpii-supp/imgidx_0472_init_graph.pdf}&
\includegraphics[width=0.16\linewidth]{figures/mpii-supp/imgidx_0472_graph.pdf}&
\includegraphics[width=0.16\linewidth]{figures/mpii-supp/imgidx_0472_sticks.pdf}\\

\includegraphics[width=0.16\linewidth]{figures/mpii-supp/imgidx_1603_init_graph.pdf}&
\includegraphics[width=0.16\linewidth]{figures/mpii-supp/imgidx_1603_graph.pdf}&
\includegraphics[width=0.16\linewidth]{figures/mpii-supp/imgidx_1603_sticks.pdf}&

  \end{tabular}
  \label{fig:qualitative_mpii_3}
\end{figure*}
