# Supplementary material for: DeepCut: Joint Subset Partition and Labeling for Multi Person Pose Estimation
Source: arXiv:1511.06645 source file (2016-04-26)
Supplement: Supplementary file 2 [file section_supplemental_mpii.tex]

\section{Additional Results on MPII Single Person dataset}

\myparagraph{PCP evaluation measure.}
